# Supplementary material for: RT-J: Large-Scale Pretraining of Relational Transformers for Context-Efficient Predictions
Source: arXiv:2610.17867 source file (2026-10-15)
Supplement: Supplementary file 1 [file rt_vs_rdblearn_body.tex]

\begin{tabular}{llrr}
\toprule
DB & Task & \rtj{} (ours, in-context) & RDBLearn (10k labels) \\
\midrule
\multicolumn{4}{l}{\textit{Regression (nMAE \%, lower is better)}} \\
\midrule
\texttt{rel-amazon} & \texttt{item-ltv} & $\mathbf{7.81}$ & $8.22$ \\
\texttt{rel-amazon} & \texttt{user-ltv} & $29.14$ & $\mathbf{25.28}$ \\
\texttt{rel-avito} & \texttt{ad-ctr} & $42.01$ & $\mathbf{35.53}$ \\
\texttt{rel-event} & \texttt{user-attendance} & $42.69$ & $\mathbf{30.97}$ \\
\texttt{rel-f1} & \texttt{driver-position} & $\mathbf{38.75}$ & $54.58$ \\
\texttt{rel-hm} & \texttt{item-sales} & $\mathbf{10.11}$ & $12.92$ \\
\texttt{rel-stack} & \texttt{post-votes} & $14.74$ & $\mathbf{13.32}$ \\
\texttt{rel-trial} & \texttt{site-success} & $89.62$ & $\mathbf{89.10}$ \\
\texttt{rel-trial} & \texttt{study-adverse} & $16.33$ & $\mathbf{12.95}$ \\
\midrule
\textbf{Mean} & & $32.35$ & $\mathbf{31.43}$ \\
\midrule
\multicolumn{4}{l}{\textit{Classification (AUROC \%, higher is better)}} \\
\midrule
\texttt{rel-amazon} & \texttt{item-churn} & $78.61$ & $\mathbf{82.07}$ \\
\texttt{rel-amazon} & \texttt{user-churn} & $67.20$ & $\mathbf{67.57}$ \\
\texttt{rel-avito} & \texttt{user-clicks} & $51.39$ & $\mathbf{69.04}$ \\
\texttt{rel-avito} & \texttt{user-visits} & $64.09$ & $\mathbf{65.49}$ \\
\texttt{rel-event} & \texttt{user-ignore} & $80.97$ & $\mathbf{82.52}$ \\
\texttt{rel-event} & \texttt{user-repeat} & $\mathbf{79.12}$ & $75.04$ \\
\texttt{rel-f1} & \texttt{driver-dnf} & $\mathbf{83.08}$ & $70.87$ \\
\texttt{rel-f1} & \texttt{driver-top3} & $\mathbf{91.00}$ & $79.69$ \\
\texttt{rel-hm} & \texttt{user-churn} & $65.66$ & $\mathbf{68.05}$ \\
\texttt{rel-stack} & \texttt{user-badge} & $81.11$ & $\mathbf{85.26}$ \\
\texttt{rel-stack} & \texttt{user-engagement} & $86.76$ & $\mathbf{89.39}$ \\
\texttt{rel-trial} & \texttt{study-outcome} & $64.43$ & $\mathbf{71.58}$ \\
\midrule
\textbf{Mean} & & $74.45$ & $\mathbf{75.55}$ \\
\bottomrule
\end{tabular}
